# Supplementary material for: Less is More: Mitigating Multimodal Hallucination from an EOS Decision Perspective
Source: arXiv:2402.14545 source file (2024-05-29)
Supplement: Supplementary file 1 [file appendix-method-1-ablation.tex]

\begin{table*}[t]
\caption{\label{tab:method-1-ablation}
CHAIR evaluation performance of models trained with different filtered data. C\(_S\) and C\(_I\) denote CHAIR\(_S\) and CHAIR\(_I\).
}
\vspace{-4pt}
\centering
\small
\begin{tabular}{@{}l|lc|cccc@{}}
\toprule
Objective & \multicolumn{1}{c}{\(y\!\neq\!v_{EOS}\)} & \(y\!=\!v_{EOS}\) & Length & CHAIR\(_S\) $\downarrow$ & CHAIR\(_I\) $\downarrow$ & Recall $\uparrow$ \\ \midrule
MLE & softmax & softmax & 100.6 & 50.0 & 15.4 & 77.1 \\
Ours & softmax\(^*\) & softmax & 79.7 & \textbf{40.2} & \textbf{12.3} & 75.7 \\
Ours\(-\) & softmax\(^*\) & - & 99.2 & 50.6 & 14.3 & \textbf{78.5} \\ \bottomrule
\end{tabular}
\end{table*}
