# Supplementary material for: Less is More: Mitigating Multimodal Hallucination from an EOS Decision Perspective
Source: arXiv:2402.14545 source file (2024-05-29)
Supplement: Supplementary file 2 [file appendix-method-2-ablation.tex]

\begin{table*}[t]
\caption{\label{tab:method-2-ablation}
CHAIR evaluation performance of models trained with different filtered data. C\(_S\) and C\(_I\) denote CHAIR\(_S\) and CHAIR\(_I\).
}
\vspace{-4pt}
\centering
\small
\begin{tabular}{@{}c|ccc|cccc@{}}
\toprule
\multirow{2}{*}{Row} & \multicolumn{3}{c|}{Train. Data} & \multicolumn{4}{c}{Model Performance} \\ \cmidrule(l){2-8} 
 & Scorer & Ratio & Length & Length & CHAIR\(_S\) $\downarrow$ & CHAIR\(_I\) $\downarrow$ & Recall $\uparrow$ \\ \midrule
1 & - & Original & 178.3 & 57.8 & 35.4 & 13.8 & 64.8 \\ \midrule
2 & \multirow{3}{*}{\(S_{final}\)} & 10\% & 171.7 & 63.7 & 35.4 & 14.0 & 64.5 \\
3 &  & 20\% & 168.2 & 45.5 & 27.0 & 10.6 & 58.9 \\
4 &  & 30\% & 166.7 & 49.2 & 29.4 & 11.7 & 58.0 \\ \midrule
5 & \multirow{3}{*}{\(S_{pos}\)} & 10\% & 181.4 & 49.4 & 29.6 & 11.2 & 57.9 \\
6 &  & 20\% & 187.2 & 46.2 & 26.8 & 11.0 & 57.9 \\
7 &  & 30\% & 194.6 & 48.3 & 30.0 & 12.4 & 57.9 \\ \midrule
8 & \(S_{neg}\) & 20\% & 164.9 & 77.2 & 38.4 & 16.1 & 65.3 \\ \bottomrule
\end{tabular}
\end{table*}
